# Supplementary material for: Measuring Distributional Shifts in Text: The Advantage of Language Model-Based Embeddings
Source: arXiv:2312.02337 source file (2023-12-04)
Supplement: Supplementary file 1 [file appendixfile.tex]

\section{Details for the experiment of Section~\ref{sec:adaptive}} \label{app:adaptive_training}

In the experiment of Section~\ref{sec:adaptive}, the model is a linear regression model with a single feature. The data it observes is i.i.d.\ Gaussian with mean zero and standard deviation one. The true labels are generated according to an linear function over the input $y = ax + b$ where $x$ is the input, $a,b$ are scalars and $y$ is the label. over time, the parameters of this generative model shift. We chose to the parameters, after every 100 examples, a Gaussian noise $\mathcal{N}(1,1)$ meaning having standard deviation 1 and mean 1. We chose a mean of 1 to make sure the model does not return to its previous state, as this is less frequent in high dimensional data. 
In our setup a system has a linear model that outputs predictions and we track the RMSE defined as the square root of the mean squared error. At any given point the system can retrain. By doing so, it updates the model to be the same as the generative model but pays a cost of 1. 

We compare two setups: (1) The first setup is called {\bf nonadaptive}, and we retrain the model at regular intervals. We control the cost, i.e., number of retrains by setting the length of the regular interval. By setting a large interval we pay a low cost but suffer a large RMSE, and conversely a small interval leads to a low RMSE but large cost; (2) The second setup is called {\bf adaptive}, and we retrain a model once its RMSE in the past 100 observations exceed some threshold. Here, this threshold is the knob we use to balance cost vs.\ RMSE. 

We repeat the following experiment with different random seeds. We draw at random which setup to use, {\bf adaptive} or {\bf nonadaptive}. We draw at random the parameter of the system, meaning the interval length for {\bf nonadaptive} and threshold for {\bf adaptive}. The model drift also behaves in an independent way in each round. Every such round provides a single triplet in the form (technique, cost, RMSE). Figure~\ref{fig:adaptive} shows a scatter plot for these points.

\section{Enabling production monitoring}\label{app:enabling}
As we describe above, we placed particular focus on making model monitoring as close to a no-code experience as possible. Users should not need to change how their model is built: we achieved this by decoupling data collection from analysis. The code to enable data collection, when using the SageMaker Python SDK, is as follows:

\begin{scriptsize}
\begin{lstlisting}[language=Python]
from sagemaker.model_monitor import DataCaptureConfig
data_capture_config = DataCaptureConfig(
    enable_capture=True,
    sampling_percentage=100,
    destination_s3_uri='s3://path/for/data/capture'
)
predictor = model.deploy(
    initial_instance_count=1,
    instance_type='ml.m4.xlarge',
    data_capture_config=data_capture_config
)
\end{lstlisting}
\end{scriptsize}

After that is done, to enable \modelmonitor/ it suffices to describe where the baseline dataset is stored, as well as the desired hardware configuration to use. 

\begin{scriptsize}
\begin{lstlisting}[language=Python]
from sagemaker.model_monitor import DefaultModelMonitor
import sagemaker.model_monitor.dataset_format as datafmt
my_monitor = DefaultModelMonitor(
    role=role,
    instance_count=1,
    instance_type='ml.m5.xlarge',
    volume_size_in_gb=20,
    max_runtime_in_seconds=3600,
)
my_monitor.suggest_baseline(
    baseline_dataset='s3://path/validation-dataset.csv',
    dataset_format=datafmt.DatasetFormat.csv(header=True),
)
\end{lstlisting}
\end{scriptsize}

Lastly, once baseline job has run, (in this case, hourly) monitoring can be enabled with:

\begin{scriptsize}
\begin{lstlisting}[language=Python]
from sagemaker.model_monitor import CronExpressionGenerator
hourly_cron = CronExpressionGenerator.hourly()
my_monitor.create_monitoring_schedule(
    monitor_schedule_name='my-monitoring-schedule',
    endpoint_input=predictor.endpoint_name,
    statistics=my_monitor.baseline_statistics(),
    constraints=my_monitor.suggested_constraints(),
    schedule_cron_expression=hourly_cron,
)
\end{lstlisting}
\end{scriptsize}
Please refer \url{https://sagemaker.readthedocs.io/en/stable/amazon_sagemaker_model_monitoring.html} for the full documentation.

\section{Sample monitoring job results}\label{app:samplereport}

We will pick regression model quality reports to illustrate here. We support standard regression metrics out of the box, and compute standard deviations by following the bootstrapping approach described in \S\ref{use-cases}.

\begin{scriptsize}
\begin{verbatim}
{
  "version" : 0.0,
  "dataset" : {
    "item_count" : 4,
    "start_time" : "2020-10-29T22:00:00Z",
    "end_time" : "2020-10-30T00:00:00Z",
    "evaluation_time" : "2021-10-13T00:17:07.894Z"
  },
  "regression_metrics" : {
    "mae" : { "value" : 0.50,  "standard_deviation" : 0.23 },
    "mse" : { "value" : 0.50, "standard_deviation" : 0.23 },
    "rmse" : { "value" : 0.71, "standard_deviation" : 0.14 },
    "r2" : { "value" : -1.67, "standard_deviation" : "NaN" }
  }
}
\end{verbatim}
\end{scriptsize}

The constraints for such data might be constructed as:

\begin{scriptsize}
\begin{verbatim}
{
  "version" : 0.0,
  "regression_constraints" : {
    "mae" : {
      "threshold" : 0.50,
      "comparison_operator" : "GreaterThanThreshold"
    },
    "mse" : {
      "threshold" : 0.50,
      "comparison_operator" : "GreaterThanThreshold"
    },
    "rmse" : {
      "threshold" : 0.71,
      "comparison_operator" : "GreaterThanThreshold"
    },
    "r2" : {
      "threshold" : -1.67,
      "comparison_operator" : "LessThanThreshold"
    }
  }
}
\end{verbatim}
\end{scriptsize}
Note that our system is designed to throw alerts if thresholds are breached when taking the standard deviation into account (e.g., for GreaterThan thresholds, only if \(value > baseline + stddev\))

\section{Sample \modelmonitor/ Visualizations}
The outputs of \modelmonitor/ can be visualized through SageMaker Studio and CloudWatch Metrics. 

\textbf{SageMaker Studio} gives the user complete access, control, and visibility into each step required to build, train, and deploy models. Users can quickly upload data, create new notebooks, train and tune models, move back and forth between steps to adjust experiments, compare results, and deploy models to production all in one place. All ML development activities including notebooks, experiment management, automatic model creation, debugging, and model and data drift detection can be performed within SageMaker Studio.

To see the \modelmonitor/ results, users can navigate to the Endpoint for which \modelmonitor/ is enabled and then select the type of monitoring results they want to view. Users can customize and add different charts to match the metrics they want to visualize. A screenshot of this view is shown in \ref{fig:studiosample}.
\begin{figure}
\centering
  \includegraphics[width=6.5cm]{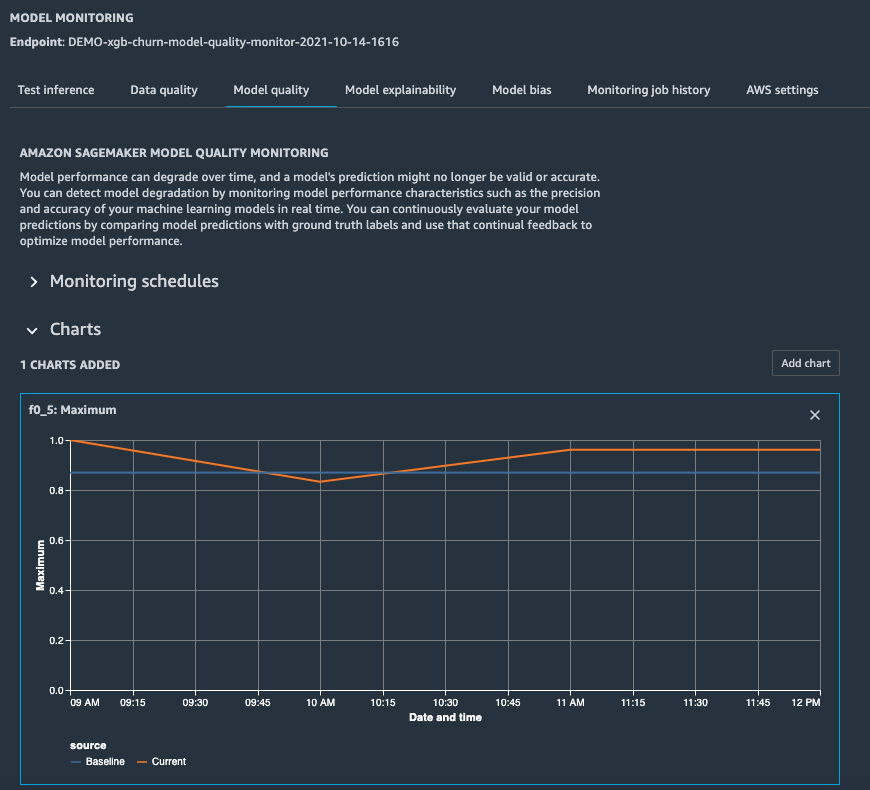}
  \caption{Model Quality tab in SageMaker Studio showing of \modelmonitor/ Model Quality calculation of the F0.5 score for a binary classification model}
  \label{fig:studiosample}
\end{figure}

\textbf{CloudWatch} provides the users with data and actionable insights to monitor applications, respond to system-wide performance changes, optimize resource utilization, and get a unified view of operational health. CloudWatch collects monitoring and operational data in the form of logs, metrics, and events, providing users with a unified view of AWS resources, applications, and services that run on AWS and on-premises servers. Users can use CloudWatch to detect anomalous behavior in your environments, set alarms, visualize logs and metrics side by side, take automated actions, troubleshoot issues, and discover insights to keep  applications
running smoothly.

\modelmonitor/ can send metrics to CloudWatch Metrics as well. Dashboards containing different graphs can be created to monitor the metrics emitted by \modelmonitor/.
In addition, CloudWatch Metrics can be configured to send a notification if metrics drop below a defined threshold. Notifications generated by CloudWatch Metrics can be used to start a retraining event.

For example, one might be interested in using \modelmonitor/ integration with Amazon SageMaker Clarify in order to improve visibility into potential bias drift. We show a sample illustration with German Credit Data dataset from UCI \cite{Dua:2019}. This dataset contains 1000 labeled credit applications and features include information concerning credit purpose, credit amount, housing status, and employment history, etc. For the sake of simplicity, categorical features are converted to indicator variables, e.g., A14 means “no checking account”. 
% We mapped the labels (Class1Good2Bad) to 0 for poor credit and 1 for good. 
As we discussed in Section \ref{sec:bias_drift}, although the initial data or model may not have been biased, changes in the world may cause bias to develop over time in a model that has already been trained. 

\begin{figure}
\centering
  \includegraphics[width=6.5cm]{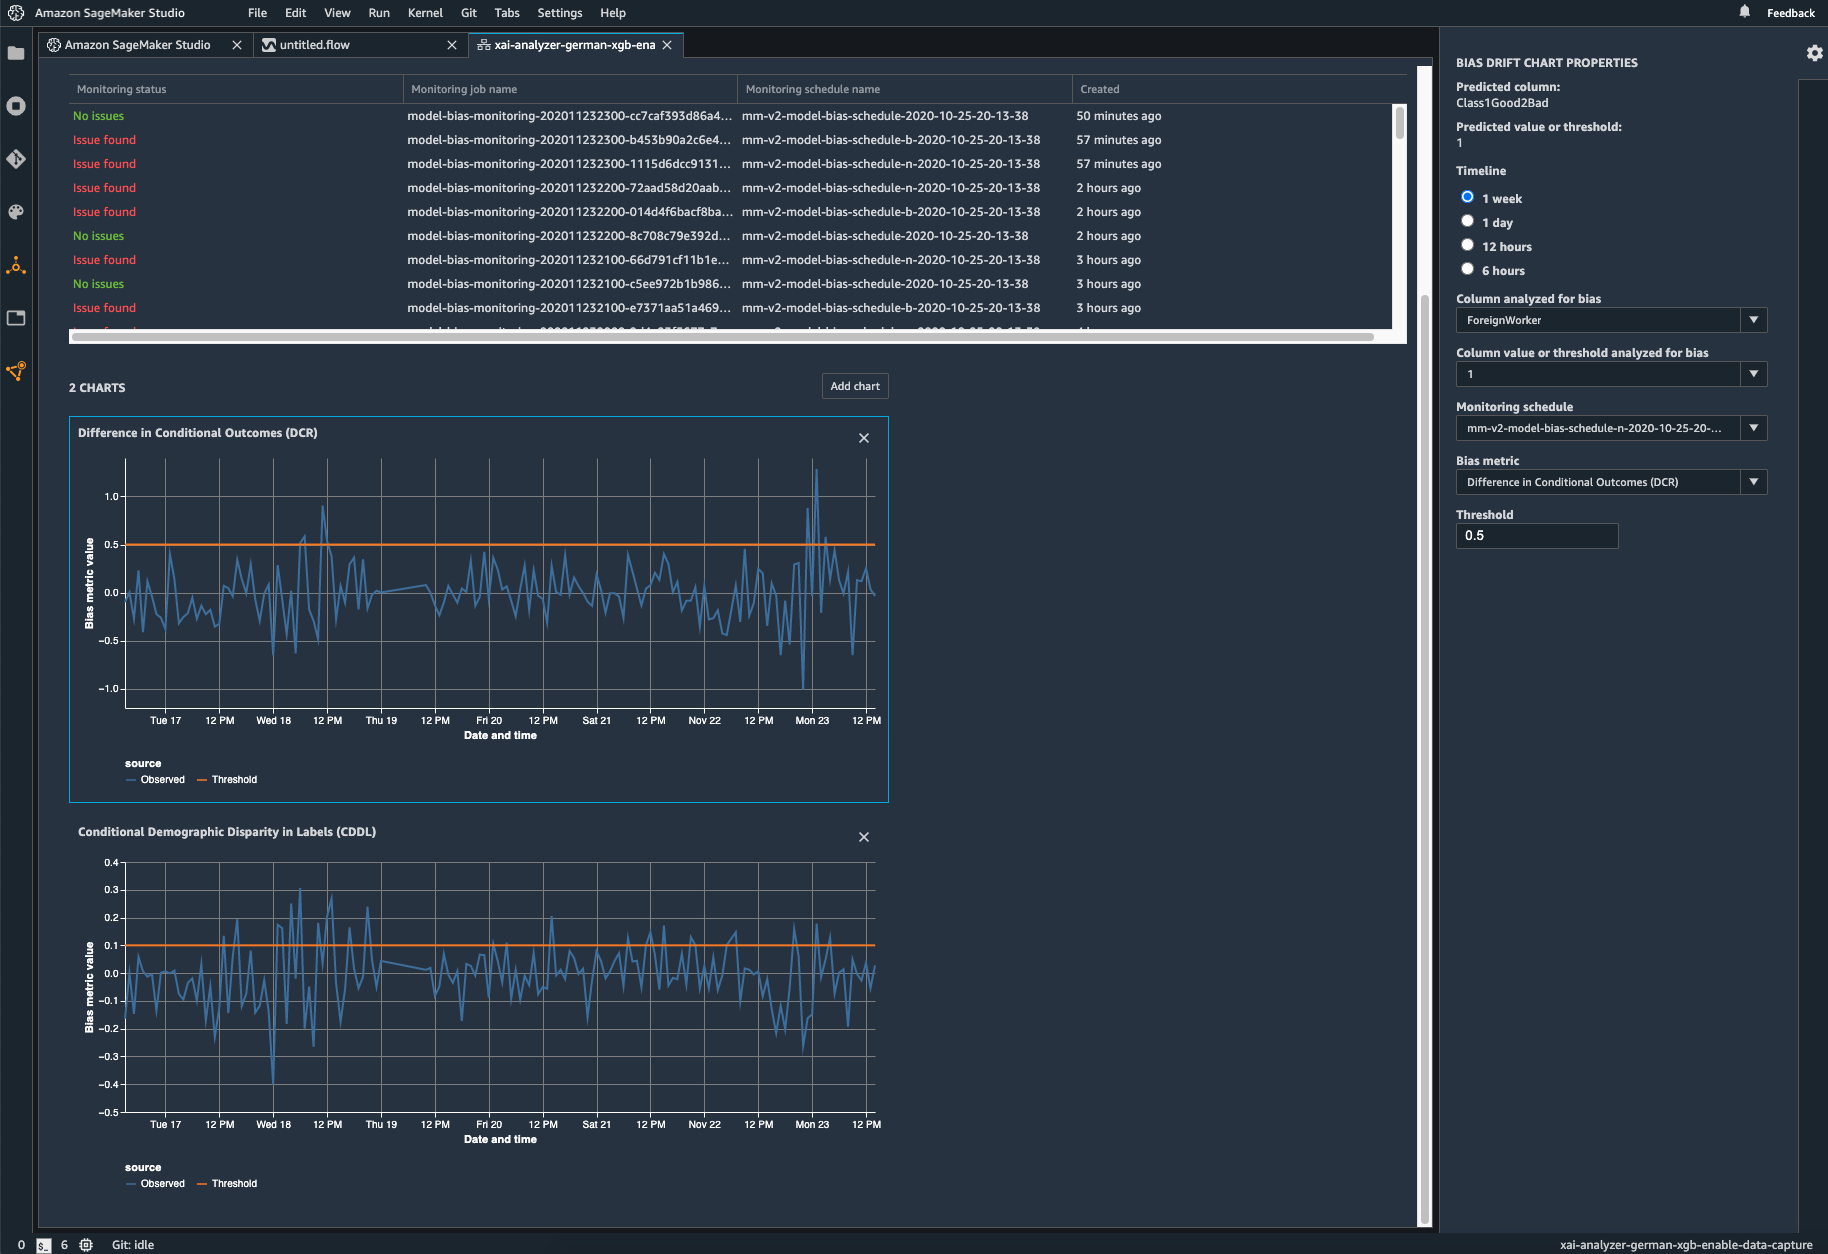}
  \caption{\modelmonitor/ controlling two bias metrics (DCR and CDDL \cite{das2021fairness}) with the feature “ForeignWorker” as sensitive attribute for German Credit Data dataset. Warnings are called when the value of the bias metrics is higher than the fixed threshold (horizontal orange lines in the monitoring plots).}
  \label{fig:german_bias_monitor}
\end{figure}

Figure \ref{fig:german_bias_monitor} shows a sample illustration of \modelmonitor/ monitoring two bias metrics (i.e., Difference in conditional rejection (DCR) and Conditional Demographic Disparity (CDDL) -- see \citet{das2021fairness} for more details) considering the feature “ForeignWorker” as sensitive attribute to protect and monitor. The system rises issues if the value of the bias metrics is higher than their fixed thresholds -- in our example 0.5 for DCR, and 0.1 for CDDL.

\begin{figure}
\centering
  \includegraphics[width=6.5cm]{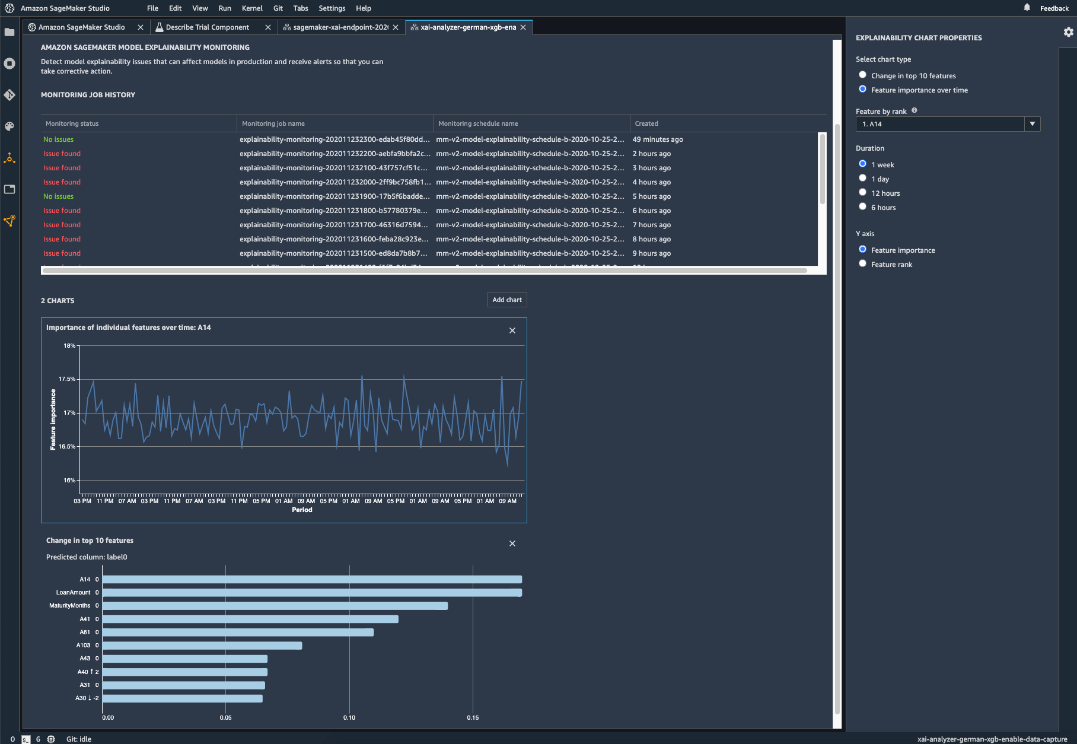}
  \caption{\modelmonitor/ analyzing the feature importance for German Credit Data dataset. Feature A14 (“no checking account”) is the most important one and \modelmonitor/ is able to analyze how the importance of feature A14 evolves through time.}
  \label{fig:german_feature_importance}
\end{figure}

Similarly, the sample illustration in Figure \ref{fig:german_feature_importance} shows the monitoring of the feature importance for German Credit Data dataset. We can note that feature A14 (“no checking account”) is the most important one and we can use \modelmonitor/ to check if the importance of feature A14 remains similar through time, or there are changes in feature importance instead.
